# Supplementary material for: Revealing the Low Temperature Phase of FAPbI$_3$ using A Machine-Learned Potential
Source: arXiv:2503.23974 ancillary file (2025-04-02)
Supplement: Supplementary file 1 [file Supporting_Information.pdf]

## Supporting Information

# Revealing the Low Temperature Phase of $FAPbI_3$ Using A Machine-Learned Potential

Sangita Dutta[1,*], Erik Fransson[1], Tobias Hainer[1], Benjamin M. Gallant[2], Dominik J. Kubicki[2], Paul Erhart[1], and Julia Wiktor[1,*]

[1]Department of Physics, Chalmers University of Technology, SE-41296, Gothenburg, Sweden
[2]School of Chamistry, University of Birmingham, Edgbaston, B15 2TT, United Kingdom

[*] sangita.dutta@chalmers.se; julia.wiktor@chalmers.se

# Supplementary Figures

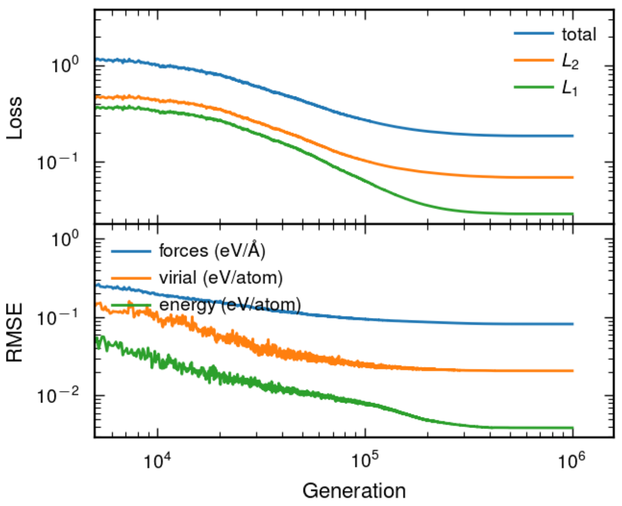


**Fig. S1:** Evolution of total loss as well as its individual contributions during training of the full model for $FAPbI_3$ based on the SCAN-VV10 functional. $L_1$, $L_2$: contribution from $L_1/_L2$-norm of parameter vector.

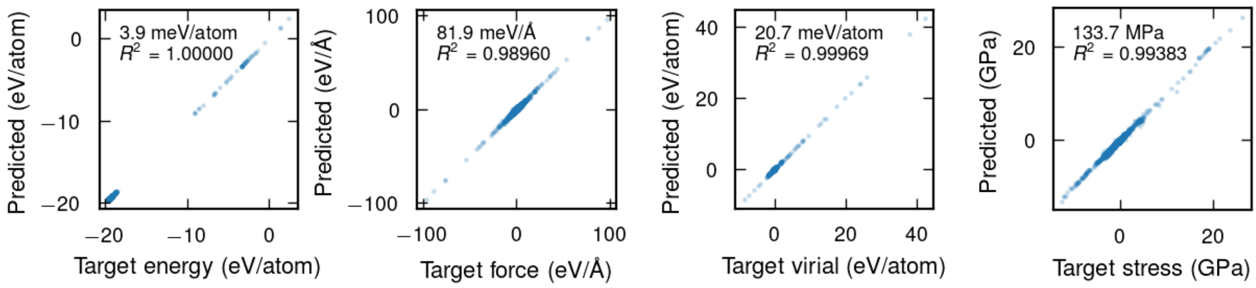


**Fig. S2:** Parity plots for total energies, forces, virials, and stresses for full model for $FAPbI_3$ based on the SCAN-VV10 functional.

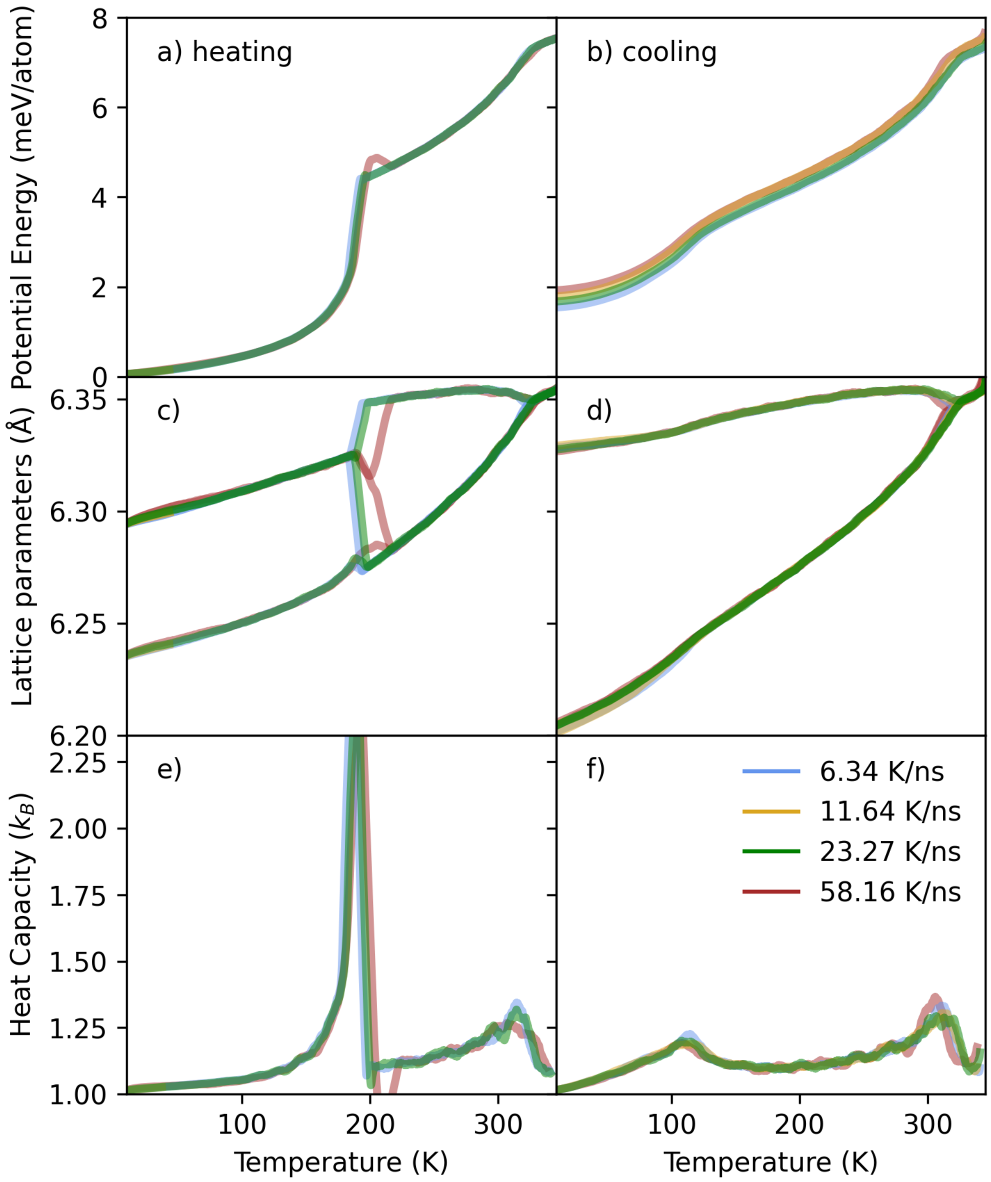


**Fig. S3:** (a) Potential energy, (b) lattice parameters, and (c) heat capacity, respectively in $FAPbI_3$ with different cooling rates. The energy difference between the structures with the highest and lowest cooling rates is 0.38 meV/atom.

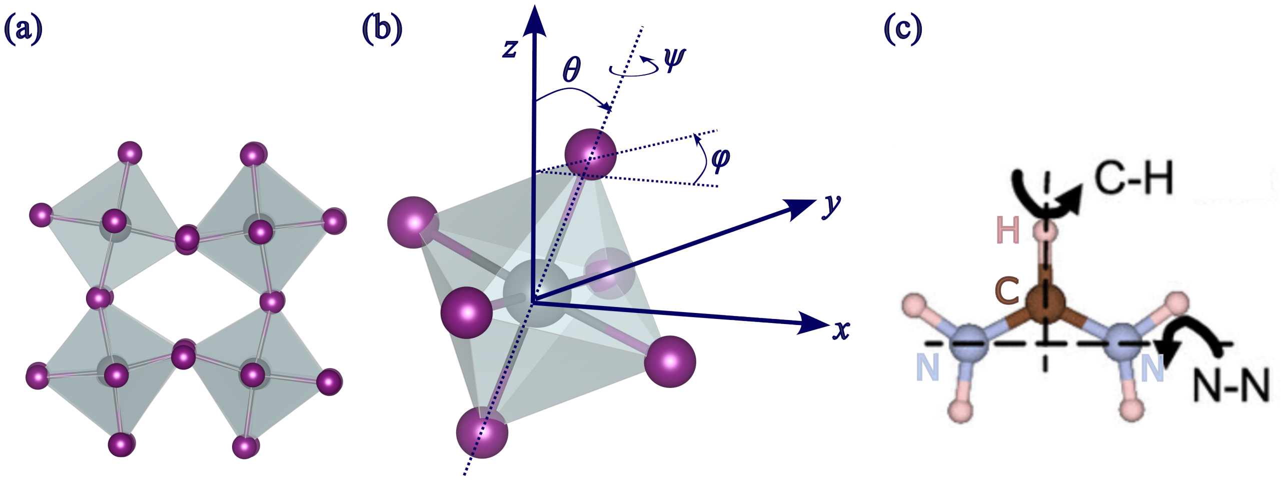


**Fig. S4:** (a) $FAPbI_3$ is represented using $PbI_6$ octahedra. (b) Define the three Euler angles $\theta$, $\phi$, and $\psi$ and describe the octahedron's orientation. (c) Represent the FA molecule indicating two rotational axis N−N, and C−H, reproduced from Ref. 1.

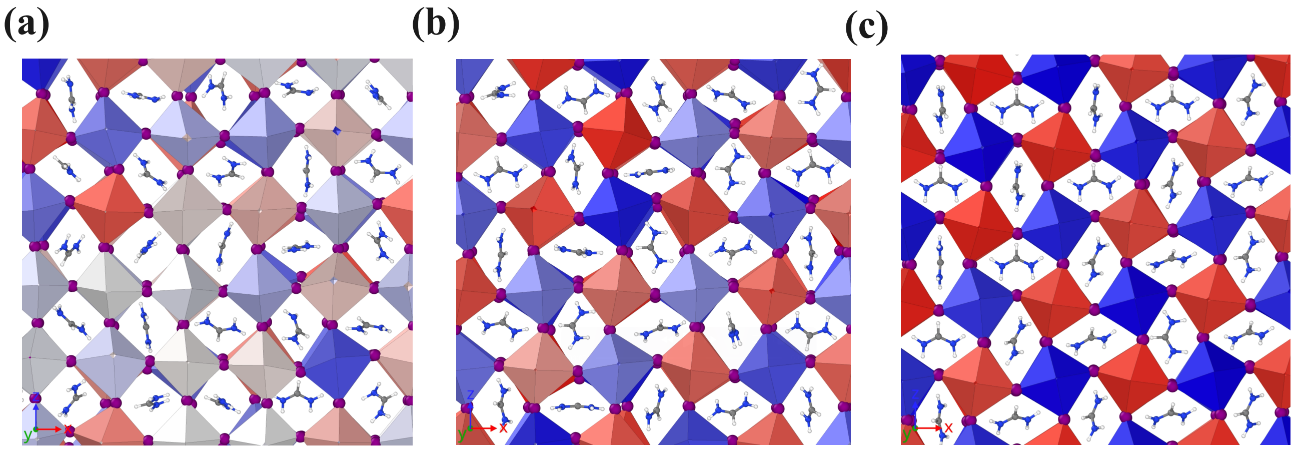


**Fig. S5:** Snapshots from the cooling molecular dynamics (MD) run, illustrating the evolution of octahedral tilts in $FAPbI_3$ at different temperatures (a) 330 K ($a^0a^0a^0$), (b) 220 K ($a^0a^0c^+$), and (c) 10 K ($a^-a^-c^+$). The color coding of the octahedra correspond to tilt angle along the z-axis (out of the screen/paper), where red corresponds to -15 and blue to 15°.

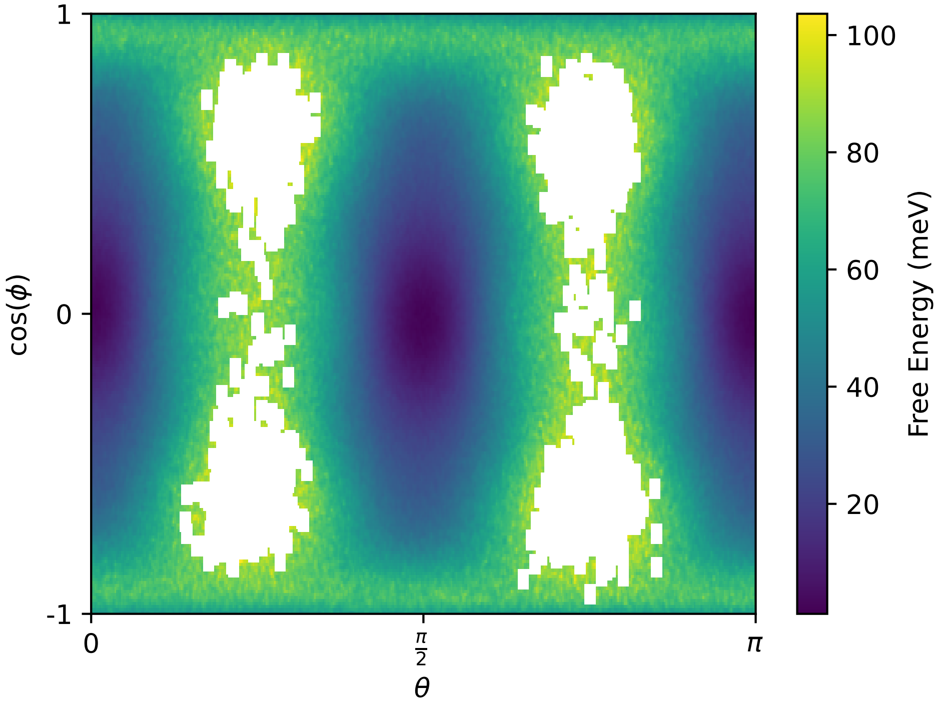


**Fig. S6:** Free energy distribution $F(\theta, \phi)$ of N−N vectors at 200 K in $a^0a^0c^+$-phase of $FAPbI_3$. Here, $\theta$ refers to angle in the $x-y$ plane and $\phi$ is angle to the $z$-axis. The white regions correspond to undefined free energy where the probability density of the N−N vectors is zero.

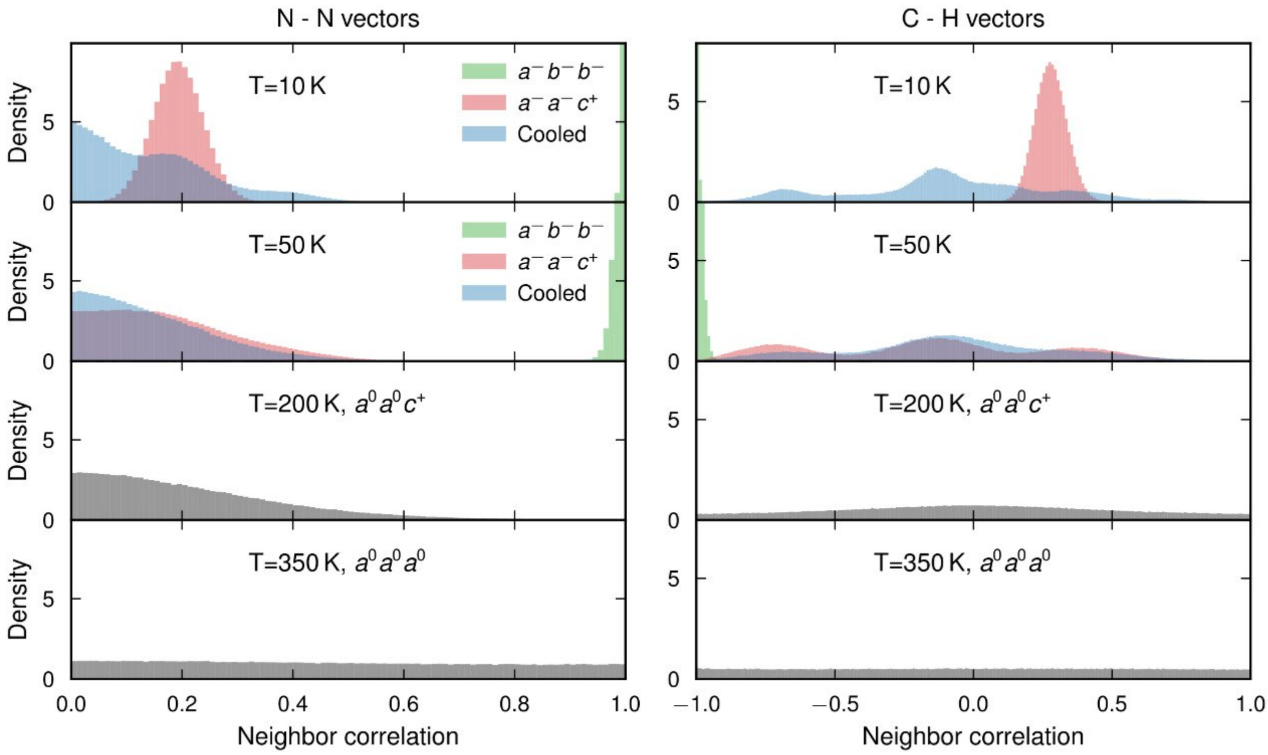


**Fig. S7:** Nearest neighbor correlation of N−N ($r^i_{NN} \cdot r^j_{NN}$ ) and C−H ($r^i_{CH} \cdot r^j_{CH}$ ) vectors in $a^-b^-b^-$ (in green), ideal $a^-a^-c^+$ (in pink) and $a^-a^-c^+$ obtained from MD cooling run (in blue), where 0 indicates two vectors are orthogonal to each other, and 1 indicates they are perfectly aligned.

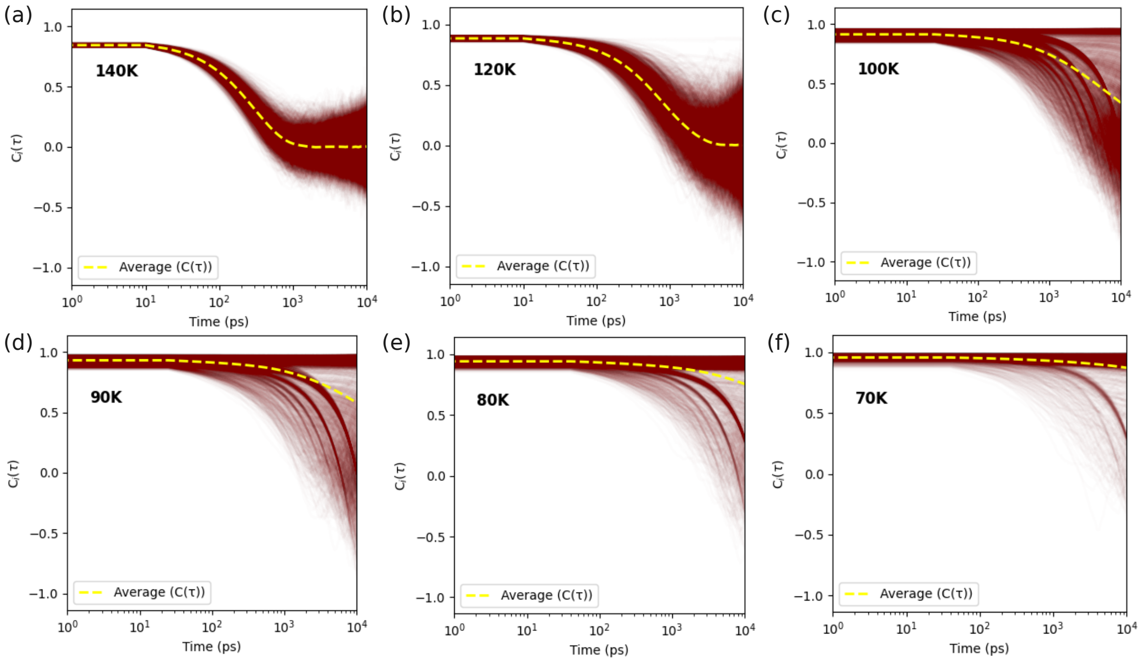


**Fig. S8:** The ACF of N−N for each FA molecule in the system as a function of time before and after second phase transition, at (a) 140 K, (b) 120 K, (c) 100 K, (d) 90 K, (e) 80 K, and (f) 70 K. The number of frozen FA molecules increases with decreasing the temperature.

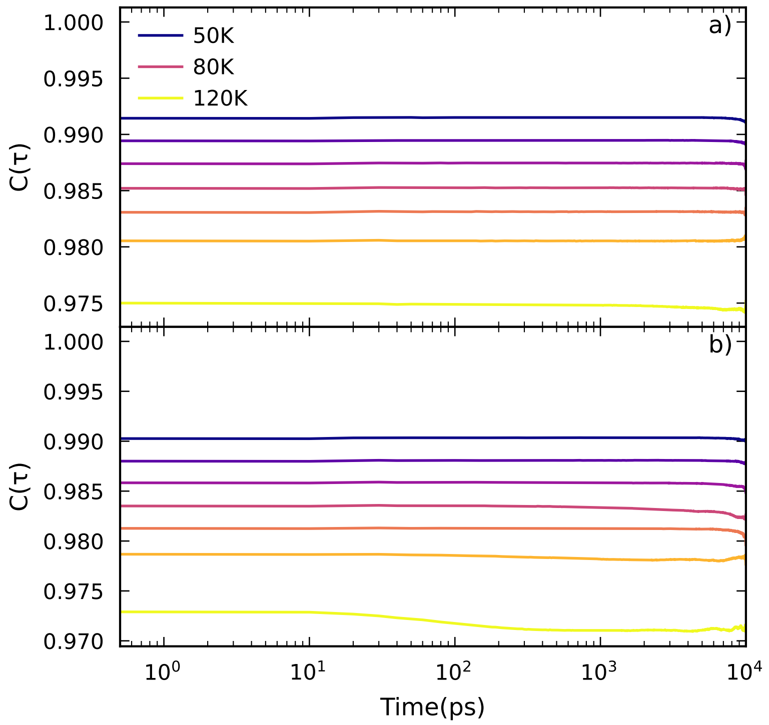


**Fig. S9:** Autocorrelation function $C(\tau)$ for the orientation of (a) N−N and (b) C−H vector in FA units in the GS phase $(a^-b^-b^-)$. The spacing between the line is 10 $K$.

# Supplementary Tables

**Table S1:** Total energies (in meV/atom) of the low-lying $FAPbI_3$ structures identified from our structural search, calculated using DFT and NEP potentials.

| Structures | DFT | | NEP | |
|---|---|---|---|---|
| | Energy | Reference Energy | Energy | Reference Energy |
| $a^-b^-b^-$ | -19.6431 | 0.0 | -19.6451 | 0.0 |
| $a^0b^-b^-$ | -19.6417 | 1.7 | -19.6445 | 0.6 |
| $a^0a^0c^+$ | -19.6394 | 3.7 | -19.6427 | 2.4 |
| $a^-a^-c^+$ | -19.6391 | 4.0 | -19.6435 | 1.6 |

**Table S2:** Summary of experimental parameters for all solid-state NMR measurements reported in this work.

| Sample | Experiment | Recycle Delay (s) | Number of Scans | Experiment Time (minutes) |
|---|---|---|---|---|
| freeze 1 | $\{^1H\}$-$^1H$-$^{13}C$ CP | 2.0 | 624 | 21 |
| | $\{^1H\}$-$^1H$-$^{15}N$ CP | 2.0 | 3400 | 116 |
| freeze 2 | $\{^1H\}$-$^1H$-$^{13}C$ CP | 2.0 | 624 | 21 |
| | $\{^1H\}$-$^1H$-$^{15}N$ CP | 2.0 | 3908 | 133 |
| freeze 3 | $\{^1H\}$-$^1H$-$^{13}C$ CP | 2.0 | 624 | 21 |
| | $\{^1H\}$-$^1H$-$^{15}N$ CP | 2.0 | 2068 | 70 |

# Supplementary References


[1] R. Lavén, M. M. Koza, L. Malavasi, A. Perrichon, M. Appel, and M. Karlsson, The Journal of Physical Chemistry Letters **14**, 2784 (2023).
